# Supplementary material for: ForeSight: Enhancing Risk Monitoring via Early Safety Signal Distillation
Source: arXiv:2609.13737 source file (2026-09-12)
Supplement: Supplementary file 1 [file appendix.tex]

\clearpage
\section{Benchmarks and Data Construction}
\label{app:benchmarks}
This section provides additional details on the benchmarks and data construction process used in our experiments.
We use safety-oriented datasets as sources of safety-sensitive prompts, and then obtain output-level harmfulness labels from the complete responses generated by each target model.
This design matches our task setting: ForeSight predicts whether the final generated response will be harmful using hidden states observed at the earliest decoding stage.




\subsection{Data Sources}

We evaluate our method on five safety-oriented datasets: HarmEval~\citep{banerjee2025safeinfer}, S-Eval~\citep{yuan2025s}, CatQA~\citep{bhardwaj2024language}, ToxicChat~\citep{lin2023toxicchat}, and WildJailbreak~\citep{jiang2024wildteaming}.
These datasets are used as sources of safety-sensitive prompts.
We retain samples that are annotated or categorized as harmful, toxic, jailbreak-related, or otherwise risk-inducing.
Importantly, these prompt-level annotations are not directly used as the prediction labels in our experiments.
Instead, the final labels are assigned according to the harmfulness of the target model's complete generated responses.

\textbf{HarmEval.}
Introduced in SafeInfer~\citep{banerjee2025safeinfer}, this policy-oriented harmfulness evaluation benchmark contains harmful prompts covering multiple prohibited-use categories and is designed to test whether language models produce unsafe responses under safety-sensitive inputs.

\textbf{S-Eval.}
This large-scale safety evaluation benchmark is organized around a hierarchical risk taxonomy~\citep{yuan2025s}. 
It includes diverse risk-inducing prompts and adversarially transformed attacks, covering areas such as illegal activities, privacy risks, hate and harassment, and unsafe advice.

\textbf{CatQA.}
This red-teaming question-answering benchmark evaluates model safety through harmful questions across a broad range of topics~\citep{bhardwaj2024language}. 
We use it to assess whether target models resist unsafe user requests.

\textbf{ToxicChat.}
Collected from real-world user interactions with a chatbot system, this toxicity benchmark provides prompts annotated for toxic and jailbreak-related content~\citep{lin2023toxicchat}. 
It is therefore useful for evaluating safety risks in realistic conversational settings.

\textbf{WildJailbreak.}
Constructed through WildTeaming, this open-source safety dataset includes harmful requests and adversarial jailbreak prompts derived from in-the-wild user-chatbot interactions~\citep{jiang2024wildteaming}. 
We use it to evaluate model behavior under jailbreak-style safety risks.

\subsection{Output-Level Label Construction}
\begin{figure}[!h]
\centering
\includegraphics[width=0.45\textwidth]{data_generation.png}
\caption{
Output-level label construction process. 
A frozen target model first generates a complete response, which is then labeled by three external judge models; only unanimous labels are retained for the main experiments.
}
\label{fig:data-generation}
\end{figure}

\begin{figure*}[!ht]
\centering
\includegraphics[width=\textwidth]{prompts.png}
\caption{
Prompt templates used for output-level labeling and text-based baseline evaluation. 
The external judge prompt labels complete generated responses, while the baseline prompt predicts final-response harmfulness from observed response prefixes.
}
\label{fig:prompt-construction}
\end{figure*}

For each prompt, we generate a complete response using a frozen target model under the same decoding configuration as in the main experiments.
During generation, we record the hidden states required by ForeSight, while the harmfulness label is assigned only after the full response has been generated.
This prevents the model from being trained on prompt-level harmfulness labels and ensures that the prediction target corresponds to the eventual safety outcome of the generated response.


We use three external judge models, Llama-3.3-70B-Instruct~\citep{grattafiori2024llama}, Mistral-Small-24B-Instruct~\citep{liu2026ministral}, and Qwen3.5-27B~\citep{team2026qwen3}, to annotate the harmfulness of each complete response.

Each complete response is assigned a binary output-level harmfulness label, where label 1 denotes a harmful response and label 0 denotes a non-harmful response. 
For each response, the judge outputs are converted into a vote count from 0 to 3, where 0 indicates that no judge labels the response as harmful and 3 indicates that all judges label the response as harmful. 
Samples with unanimous judgments, i.e., vote counts of 0 or 3, are used for the main experiments, while non-unanimous samples with vote counts of 1 or 2 are treated as borderline cases for additional analysis.
After removing non-unanimous samples, we split the remaining data into training, validation, and test sets with an 8:1:1 ratio.

\begin{table}[t]
\centering
\small
\setlength{\tabcolsep}{8pt}
\renewcommand{\arraystretch}{1.2}
\begin{tabular}{lccccc}
\toprule
\textbf{Model} & \textbf{0} & \textbf{1} & \textbf{2} & \textbf{3} & \textbf{Total} \\
\midrule

\rowcolor[gray]{0.9} \multicolumn{6}{l}{\textbf{HarmEval}} \\
Llama3.1-8B    & 269 & 62  & 60  & 159 & 550 \\
Qwen3-8B       & 458 & 46  & 37  & 9   & 550 \\

\rowcolor[gray]{0.9} \multicolumn{6}{l}{\textbf{S-Eval}} \\
Llama3.1-8B    & 553 & 123 & 85  & 239 & 1000 \\
Qwen3-8B       & 830 & 64  & 54  & 52  & 1000 \\

\rowcolor[gray]{0.9} \multicolumn{6}{l}{\textbf{CatQA}} \\
Llama3.1-8B    & 152 & 95  & 47  & 256 & 550 \\
Qwen3-8B       & 504 & 16  & 21  & 9   & 550 \\

\rowcolor[gray]{0.9} \multicolumn{6}{l}{\textbf{ToxicChat}} \\
Llama3.1-8B    & 9112 & 366 & 202 & 232 & 9912 \\
Qwen3-8B       & 9532 & 198 & 110 & 78  & 9918 \\

\rowcolor[gray]{0.9} \multicolumn{6}{l}{\textbf{WildJailbreak}} \\
Llama3.1-8B    & 353 & 75  & 69  & 153 & 650 \\
Qwen3-8B       & 429 & 55  & 61  & 115 & 660 \\

\bottomrule
\end{tabular}
\caption{Distribution of harmfulness vote counts across datasets and target models. Columns 0--3 denote the number of judge models that label the generated response as harmful.}
\label{tab:label-distribution}
\end{table}

The totals may differ slightly across target models because a small number of judge outputs cannot be parsed into a valid label and are therefore excluded before aggregation.
The non-unanimous cases, corresponding to vote counts of 1 or 2, are not used as the primary training or evaluation labels, but are further analyzed as borderline cases.




\begin{figure*}[!ht]
\centering
\includegraphics[width=\textwidth]{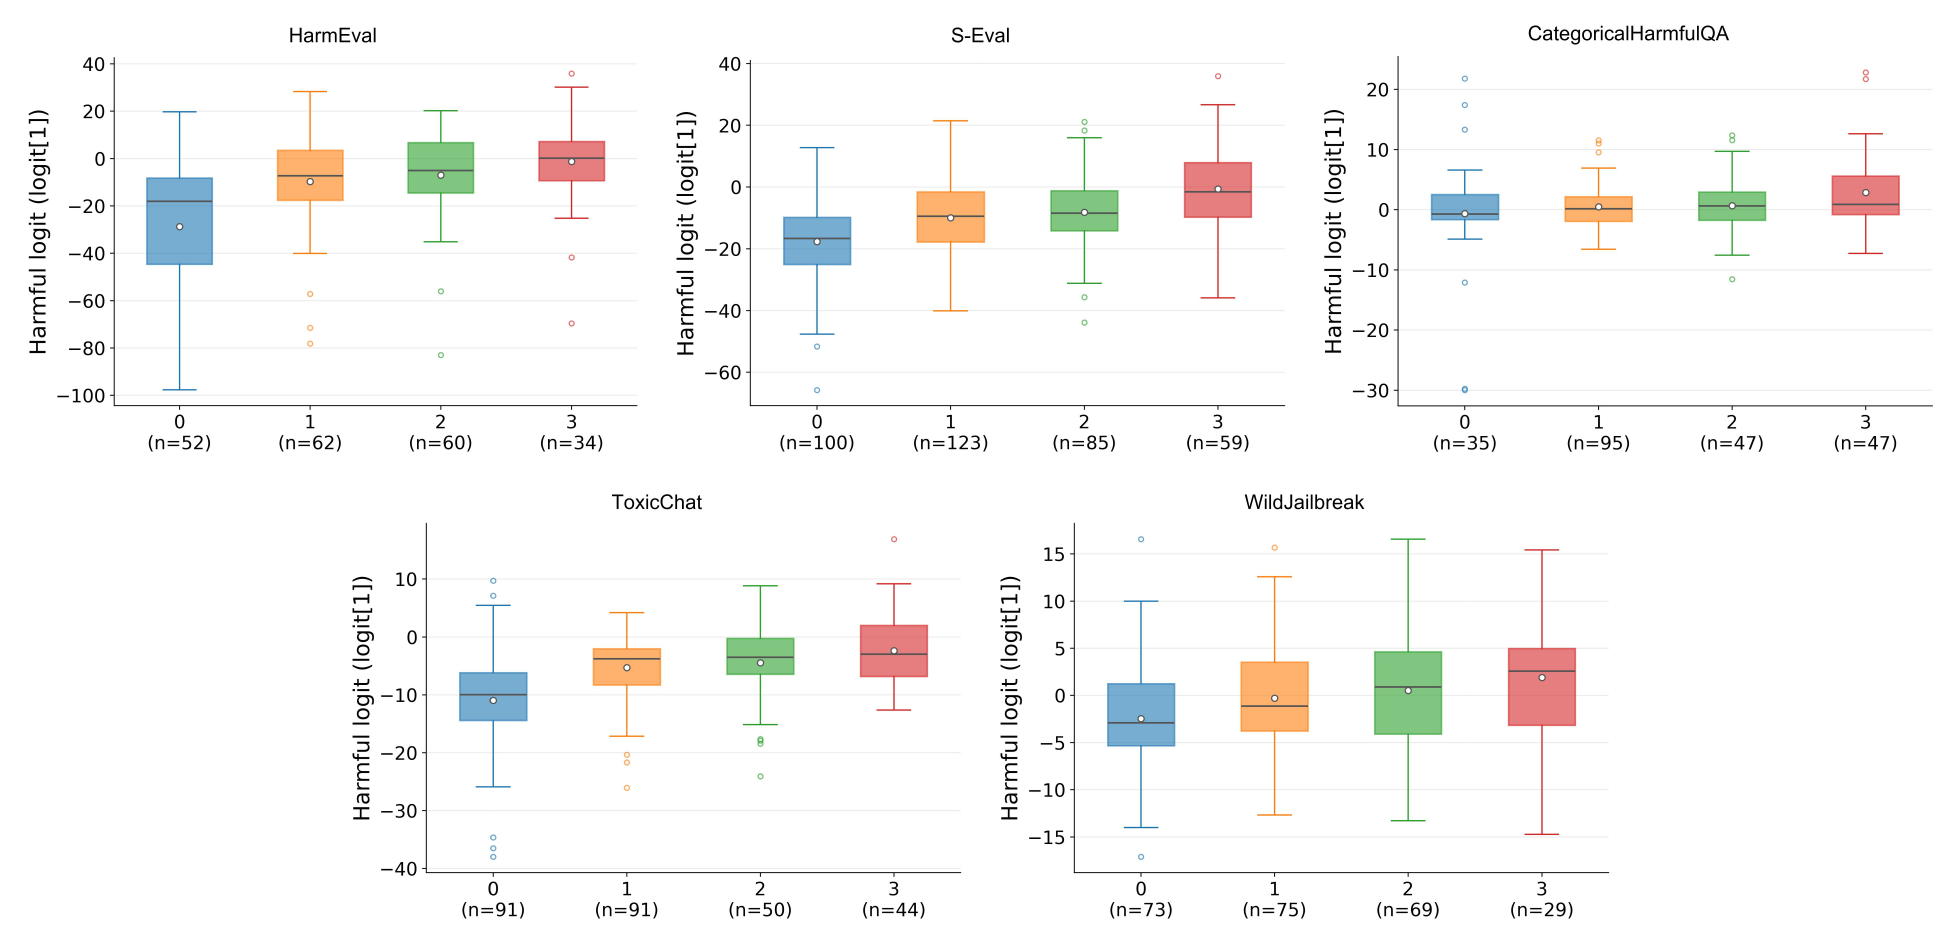}
\caption{Borderline cases with non-unanimous harmfulness judgments.}
\label{fig:borderline}
\end{figure*}




\section{Detailed Baseline Settings}
\label{app:baseline_setting}

We provide detailed descriptions of the baselines used in our evaluation.
Since our task focuses on early harmfulness forecasting, all baselines are evaluated under an early-observation setting and are required to predict whether the final generated response will be harmful.

\subsection{Text-based Baselines}

For text-based baselines, the observable input consists of the original prompt and the first 10 generated tokens.
All models are evaluated using the same prompt template, as shown in Figure~\ref{fig:prompt-construction}.

\textbf{Llama-3.3-70B-Instruct.}
Llama-3.3-70B-Instruct is a large instruction-tuned language model from the Llama family~\citep{grattafiori2024llama}.
We use it as a judge-style safety classifier to assess whether strong general-purpose LLMs can forecast output harmfulness from a short generated prefix.

\textbf{Mistral-Small-24B-Instruct.}
Mistral-Small-24B-Instruct is an instruction-tuned model from the Mistral family~\citep{liu2026ministral}.
It serves as another large judge-style baseline for early harmfulness classification.

\textbf{Qwen3.5-27B.}
Qwen3.5-27B is a large instruction-tuned model from the Qwen family~\citep{team2026qwen3}.
Together with the above judge models, it provides a strong text-based reference for early output-level harmfulness prediction.

\textbf{LlamaGuard3-8B.}
LlamaGuard3-8B is an open-source safety guardrail model designed for content moderation~\citep{inan2023llama}.
Unlike general judge models, it is specifically trained for safety classification, and its output is converted into a binary harmfulness label.

\textbf{Qwen3Guard-8B.}
Qwen3Guard-8B is a safety guardrail model from the Qwen family~\citep{zhao2025qwen3guard}.
We use it as another open-source moderation baseline with a comparable safety-classification objective.

\subsection{Method-based Baselines}
We follow their original feature extraction while evaluating it on our benchmark splits.

\textbf{MULI.}
MULI is a logits-based early forecasting method for predicting response harmfulness from early decoding signals~\citep{hu2024toxicity}.
Instead of relying on an external judge model, it uses output logits produced during generation as features for harmfulness prediction.


\textbf{Latent Guard.}
Latent Guard is a hidden-state-based safety forecasting method that detects harmfulness using internal representations of the language model~\citep{zhao2026llms}.
It is closely related to our setting because it leverages latent model states rather than surface text alone.









\begin{figure*}[!h]
\centering
\includegraphics[width=\textwidth]{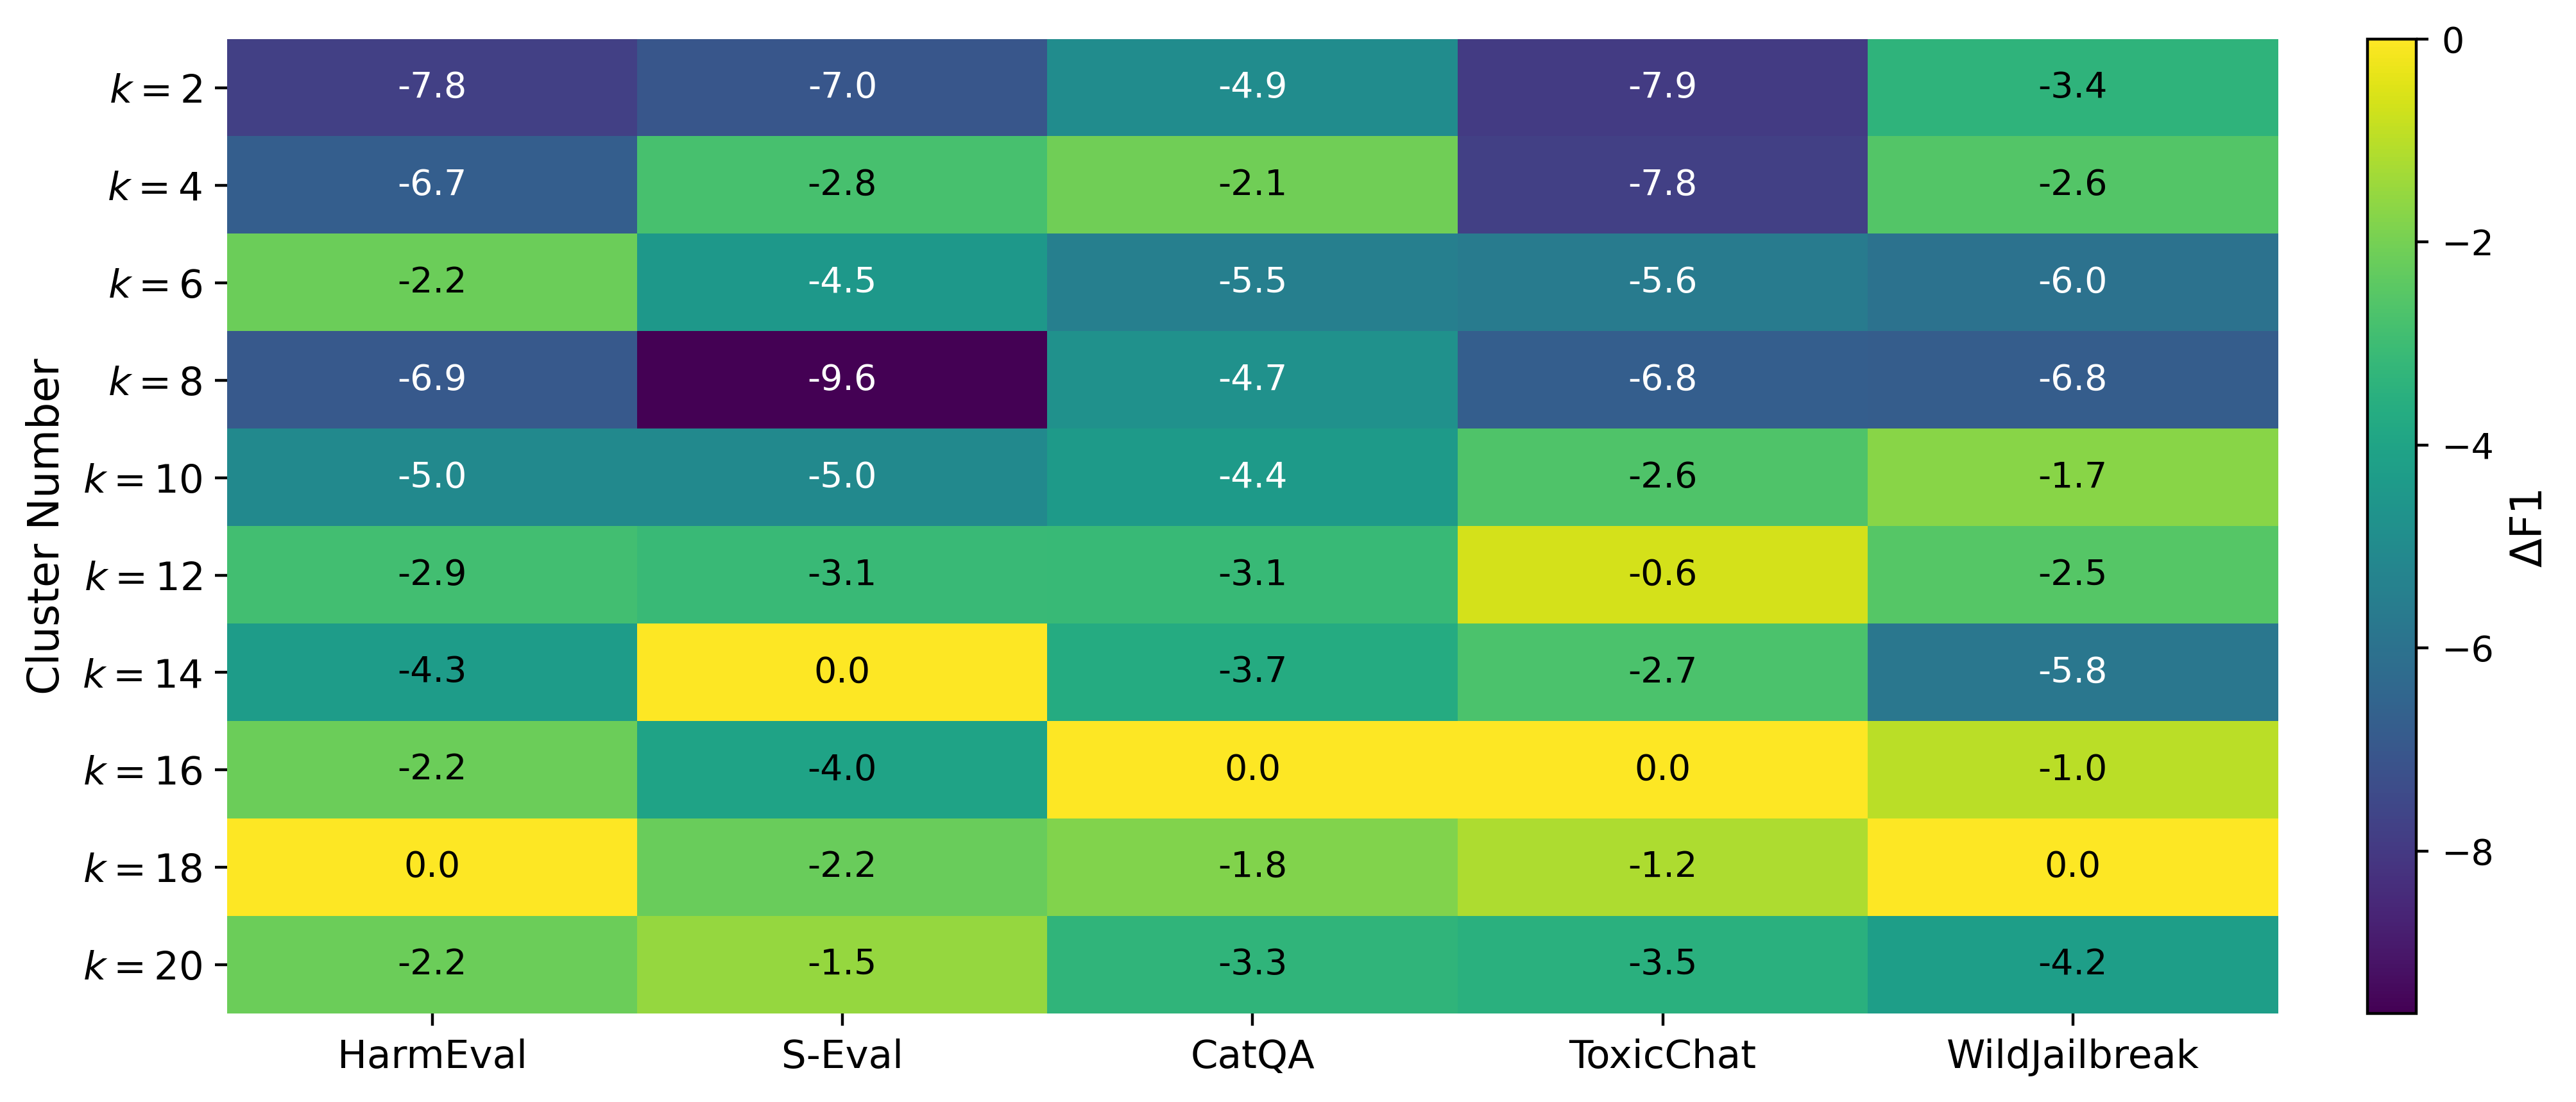}
\caption{Effect of the cluster number $k$ of Llama3.1-8B across datasets. Values denote $\Delta$F1 relative to the dataset-specific best result.}
\label{fig:transferability}\end{figure*}



\section{Experimental Settings and Hyperparameters}
\label{app:hyperparameters}

This section summarizes the implementation settings and hyperparameters used for ForeSight. 
The layer-wise L1 regularization strength and the number of K-means clusters are selected based on validation performance.

\begin{table}[t]
\centering
\small
\setlength{\tabcolsep}{8pt}
\renewcommand{\arraystretch}{1.15}
\begin{tabular}{lc}
\toprule
\textbf{Item} & \textbf{Setting} \\
\midrule
Observation window & First generated token \\
Neuron saliency threshold & 0.35 \\
L1 regularization search range & $\{100, 200, \ldots, 2000\}$ \\
K-means cluster search range & $\{2, 4, \ldots, 20\}$ \\
Selection criterion & Validation performance \\
Training batch size & 32 \\
Hardware & 4 NVIDIA A800 GPUs \\
\bottomrule
\end{tabular}
\caption{Implementation settings and hyperparameters for ForeSight experiment.}
\label{tab:hyperparameters}
\end{table}
 



% 如果你没有 Spearman/Pearson 数值，就不要写 strong correlation，可以写 positive association / clear increasing trend / generally increase，更稳。

\section{Cluster Number Transferability}
\label{app:cluster_transferability}
We further examine the effect of the cluster number $k$ across different datasets.
As shown in Figure~\ref{fig:transferability}, the optimal value of $k$ is not identical across benchmarks, suggesting that the most suitable clustering granularity can vary with the data distribution.
However, the high-performing region is relatively concentrated.
Most datasets achieve their best or near-best results when $k$ falls between 14 and 18, while overly small values of $k$ often lead to larger performance drops.

This pattern indicates that the clustering module does not require an exact globally fixed cluster number, but it benefits from a moderate level of granularity.
When $k$ is too small, neurons with different safety-related activation patterns may be merged into the same cluster, weakening the discriminative signal after aggregation.
In contrast, moderate-to-large values preserve more fine-grained structure and generally produce more stable performance across datasets.
Therefore, in our main experiments, we do not impose a universal fixed $k$ for all settings; instead, $k$ is selected according to validation performance.
The results show that this selection is well-behaved, as competitive values consistently lie within a narrow and interpretable range.



\section{Case Study}

\subsection{Borderline Evaluation}


In the main experiments, we retain only samples with unanimous evaluator labels to reduce annotation noise, as summarized in Table~\ref{tab:label-distribution}. 
While this protocol improves label reliability, it may also remove borderline cases whose harmfulness is inherently ambiguous. 
To address this concern, we conduct an additional analysis on the non-unanimous samples that are excluded from the main training and evaluation splits.

For each non-unanimous sample, we define the harmfulness vote rate as the proportion of evaluators that assign a harmful label. 
We then compare this vote rate with the harmfulness score predicted by ForeSight, obtained from the classifier logits after normalization. 
As shown in Figure~\ref{fig:borderline}, samples with higher harmfulness vote rates generally receive higher predicted harmfulness scores. 
This suggests that ForeSight does not merely separate easy harmful and harmless cases, but also captures graded early safety signals in ambiguous responses.


\subsection{Failure Case Analysis}

\begin{figure}[!h]
\centering
\includegraphics[width=0.5\textwidth]{failure_case.png}
\caption{Distribution of ForeSight failure categories in the borderline test subset.}
\label{fig:failure-case}
\end{figure}

\begin{table*}[t]
\centering
\small
\setlength{\tabcolsep}{5pt}
\renewcommand{\arraystretch}{1.15}
\begin{tabular}{p{0.18\linewidth}p{0.13\linewidth}p{0.13\linewidth}p{0.25\linewidth}p{0.25\linewidth}}
\toprule
\textbf{Failure Type} 
& \textbf{Ground Truth} 
& \textbf{Prediction} 
& \textbf{Representative Pattern} 
& \textbf{Interpretation} \\
\midrule

Input-dominant FP 
& 0
& 1
& A safety-sensitive prompt is followed by a safe, evasive, or non-substantive response. 
& Early hidden states may over-emphasize input-level risk rather than the harmfulness of the final response. \\

Ambiguity-masked FN 
& 1
& 0 
& The response contains harmful content, but it is preceded or followed by disclaimers, warnings, or hedging expressions. 
& Surface-level safety language may obscure the harmfulness of the substantive content, making the early signal less decisive. \\

Jailbreak-induced FN 
& 1
& 0 
& The user prompt uses jailbreak-style framing, such as role-play, hypothetical scenarios, multi-turn persuasion, or task reframing, to elicit harmful content. 
& Jailbreak framing can make the generation context appear less directly harmful, weakening the early separation between harmful and non-harmful outputs. \\

Other output-harmful FN 
& 1
& 0 
& The response is labeled harmful, but its surface form is ambiguous or does not match common instruction-like harmful patterns. 
& Some harmful outputs may not align well with the safety features learned from more direct harmful cases. \\

\bottomrule
\end{tabular}

\caption{Macro-level failure categories of ForeSight.}
\label{tab:badcase}

\vspace{1mm}
\begin{minipage}{0.96\textwidth}
\footnotesize
\textit{Note:} 
In this table, 1 denotes a harmful output and 0 denotes a non-harmful output. 
Thus, FP refers to non-harmful outputs incorrectly predicted as harmful, whereas FN refers to harmful outputs missed by the detector.
\end{minipage}
\end{table*}

As shown in Figure~\ref{fig:failure-case} and Table~\ref{tab:badcase}, input-dominant false positives form the largest group of errors.
These cases occur when the prompt is clearly safety-sensitive, but the generated response is ultimately safe, evasive, or non-substantive.
This suggests that first-token hidden states may sometimes encode the risk profile of the user request more strongly than the harmfulness of the final response.

False negatives show a different pattern.
In ambiguity-masked cases, the final response still contains harmful content, but such content is mixed with disclaimers, warnings, or hedging expressions.
Although these surface-level safety markers make the response appear less explicitly harmful, they do not necessarily remove the harmful substance of the output.
This indicates that early hidden states may be less decisive when harmful assistance is partially obscured by safety-oriented language.

We also observe jailbreak-induced false negatives, where the user prompt relies on role-play, hypothetical scenarios, multi-turn persuasion, or task reframing to elicit harmful content.
Compared with direct harmful requests, these prompts create a less explicit generation context, making the early representation harder to separate from benign explanatory or fictional text.
Finally, other output-harmful false negatives correspond to harmful responses whose surface forms are atypical or weakly aligned with the more direct harmful patterns seen during training.
We additionally identify 61 near-boundary cases with small logit margins, which are treated as an overlapping attribute rather than a separate failure type.








% \paragraph{Lexical Cue Analysis.}
% To further summarize the surface patterns associated with model errors, we visualize the most frequent lexical cues in false-positive and false-negative cases...
